# Supplementary material for: Solving Vlasov Equations Using NRxx Method
Source: arXiv:1209.0527 source file (2012-09-04)
Supplement: Supplementary file 1 [file article_appendix.tex]

% vim: tw=70:spell
\section*{Appendix}

\appendix

\section{Some properties of Hermite polynomials} \label{sec:Hermite}
The Hermite polynomials defined in \eqref{eq:He} are a set of
orthogonal polynomials over the domain $(-\infty, +\infty)$. Their
properties can be found in many mathematical handbooks such as \cite
{Abramowitz}. Some useful ones are listed below:
\begin{enumerate}
\item Orthogonality: $\displaystyle \int_{\bbR} \He_m(x)
\He_n(x) \exp(-x^2/2) \dd x = m! \sqrt{2\pi} \delta_{m,n}$;
\item Recursion relation: $\He_{n+1}(x) = x \He_n(x) - n \He_{n-1}(x)$;
\item Differential relation: $\He_n'(x) = n \He_{n-1}(x)$.
\end{enumerate}
And the following equality can be derived from the last two relations:
\begin{equation}
[\He_n(x) \exp(-x^2/2)]' = -\He_{n+1}(x) \exp(-x^2/2).
\end{equation}

\section{Derivation of the moment equations} \label{sec:moment_eqs}
In order to derive the analytical form of the moment equations, we
need to put the expanded distribution \eqref{eq:expansion} into the
Boltzmann-BGK equation \eqref{eq:BGK}. The subsequent calculation will
involve the temporal and spatial differentiation of the basis function
$\mathcal{H}_{\theta,\alpha}(\bv)$, which will be first calculated as
\begin{equation} \label{eq:dHds}
\begin{split}
  \pdd{s}\mathcal{H}_{\theta,\alpha}(\bv)& = -
    \frac{|\alpha|+D}{2}(2\pi)^{-\frac{D}{2}}
    \theta^{-\frac{|\alpha|+D}{2}-1}
    \pd{\theta}{s} \prod_{d=1}^D \He_{\alpha_d}(v_d) 
    \exp\left(-\frac{v_d^2}{2}\right) \\
  & \quad -(2\pi)^{-\frac{D}{2}}\theta^{-\frac{|\alpha|+D}{2}}
    \sum_{j=1}^{D} \left[\pd{v_{j}}{s} 
    \prod_{d=1}^{D} \He_{\alpha_{d} +\delta_{jd}}(v_d) 
    \exp\left(-\frac{v_d^2}{2}\right)\right] \\ 
  &= -\frac{|\alpha|+D}{2\theta} \pd{\theta}{s}
    \mathcal{H}_{\theta,\alpha}(\bv) -
    \sqrt{\theta}\sum_{d=1}^{D} \pd{v_{d}}{s}
    \mathcal{H}_{\theta,\alpha+e_{d}}(\bv),
\end{split}
\end{equation}
where $s$ stands for $t$ or $x_j$, $j = 1,2,3$. The partial derivative
$\partial v_d / \partial s$ can be expanded as
\begin{equation} \label{eq:dvds}
  \pd{v_d}{s} = \pdd{s}\left(\frac{\xi_d -u_d}{\sqrt{\theta}}\right)
    = -\frac{1}{\sqrt{\theta}}\pd{u_d}{s} -
      \frac{v_d}{2\theta} \pd{\theta}{s}.
\end{equation}
Noting that the recursion of the Hermite polynomials gives
\begin{equation} \label{eq:vH}
v_d \mathcal{H}_{\theta, \alpha+e_d}(\bv) =
  \sqrt{\theta} \mathcal{H}_{\theta, \alpha + 2e_d}(\bv) +
  \frac{\alpha_d + 1}{\sqrt{\theta}} \mathcal{H}_{\theta, \alpha}(\bv),
\end{equation}
we conclude from \eqref{eq:dHds}, \eqref{eq:dvds} and \eqref{eq:vH}
that
\begin{equation} \label{eq:dHds1}
\pdd{s} \mathcal{H}_{\theta,\alpha}(\bv) =
  \sum_{d=1}^D\pd{u_d}{s}
  \mathcal{H}_{\theta,\alpha+e_{d}}(\bv)+\frac{1}{2}\pd{\theta}{s}
  \sum_{d=1}^D \mathcal{H}_{\theta,\alpha+2e_d}(\bv).
\end{equation}
Replacing $s$ with $t$ in the above equation, one can have the
following expansion of the time derivative term in the Boltzmann-BGK
equation \eqref{eq:BGK} by some simple calculation:
\begin{equation} \label{eq:time_diff}
\begin{split}
\pd{f}{t} &= \sum_{\alpha \in \bbN^D} \left(
    \pd{f_{\alpha}}{t} \mathcal{H}_{\theta,\alpha} +
    f_{\alpha} \pd{\mathcal{H}_{\theta,\alpha}}{t}
  \right) \\
& = \sum_{\alpha \in \bbN^D} \left(
    \pd{f_{\alpha}}{t} + \sum_{d=1}^D \pd{u_d}{t} f_{\alpha-e_{d}}
    + \frac{1}{2} \pd{\theta}{t} \sum_{d =1}^D f_{\alpha-2e_d}
  \right) \mathcal{H}_{\theta,\alpha}.
\end{split}
\end{equation}
Now we consider the convection term. Substituting $x_j$ for $s$ in
\eqref{eq:dHds1}, and making use of \eqref{eq:vH} again, one has
\begin{equation} \label{eq:convection}
\begin{split}
\nabla_{\bx}\cdot(\bxi f) &= \sum_{j=1}^D \xi_j \pd{f}{x_j}
  = \sum_{j=1}^D (u_j + \sqrt{\theta} v_j)
    \sum_{\alpha \in \bbN^D} \left(
      \pd{f_{\alpha}}{x_j} \mathcal{H}_{\theta,\alpha} +
      f_{\alpha} \pd{\mathcal{H}_{\theta,\alpha}}{x_j}
    \right) \\
& = \sum_{\alpha \in \bbN^D}
  \mathcal{H}_{\theta,\alpha} \sum_{j=1}^D \bigg[ \left(
    \theta \pd{f_{\alpha-e_{j}}}{x_{j}} +
    u_{j}\pd{f_{\alpha}}{x_j} +
    (\alpha_{j}+1)\pd{f_{\alpha+e_j}}{x_{j}}
  \right) \\
& \qquad {} + \sum_{d=1}^D \pd{u_d}{x_j} \left(
  \theta f_{\alpha-e_d-e_j} + u_j f_{\alpha-e_d}
  + (\alpha_{j}+1) f_{\alpha-e_d+e_j}
\right) \\
& \qquad {} + \frac{1}{2} \pd{\theta}{x_j}
  \sum_{d=1}^D \left( \theta f_{\alpha-2e_d-e_j} +
  u_j f_{\alpha-2e_d} + (\alpha_{j}+1) f_{\alpha-2e_d+e_j}
\right) \bigg].
\end{split}
\end{equation}
Using $f_M = f_0 \mathcal{H}_{\theta,0}(\bv)$, the relaxation term can
be simply expanded as
\begin{equation} \label{eq:collision}
\frac{1}{\tau} (f_M - f) =
  -\frac{1}{\tau} \sum_{|\alpha| \geqslant 1}
  f_{\alpha} \mathcal{H}_{\theta,\alpha}(\bv).
\end{equation}

Finally, we combine \eqref{eq:time_diff}, \eqref{eq:convection} and
\eqref{eq:collision} and find the ultimate moment equations as
\begin{equation} \label{eq:moment_eqs}
\begin{split}
& \left( \pd{f_{\alpha}}{t} +
  \sum_{d=1}^D \pd{u_d}{t} f_{\alpha-e_{d}}
  + \frac{1}{2} \pd{\theta}{t} \sum_{d =1}^D f_{\alpha-2e_d}
  \right) \\
& \qquad + \sum_{j=1}^D \bigg[ \left(
  \theta \pd{f_{\alpha-e_{j}}}{x_{j}} +
  u_{j}\pd{f_{\alpha}}{x_j} +
  (\alpha_{j}+1)\pd{f_{\alpha+e_j}}{x_{j}}
\right) \\
& \qquad {} + \sum_{d=1}^D \pd{u_d}{x_j} \left(
  \theta f_{\alpha-e_d-e_j} + u_j f_{\alpha-e_d}
  + (\alpha_{j}+1) f_{\alpha-e_d+e_j}
\right) \\
& \qquad {} + \frac{1}{2} \pd{\theta}{x_j}
  \sum_{d=1}^D \left( \theta f_{\alpha-2e_d-e_j} +
  u_j f_{\alpha-2e_d} + (\alpha_{j}+1) f_{\alpha-2e_d+e_j}
\right) \bigg] = -\frac{1 - \delta_{0\alpha}}{\tau} f_{\alpha},
\end{split}
\end{equation}
where $\alpha \in \bbN^D$ and 
\begin{equation}
\delta_{0\alpha} = \left\{ \begin{array}{ll}
  1, & \alpha = 0, \\
  0, & \text{otherwise}.
\end{array} \right.
\end{equation}
